# Supplementary material for: Analysis and Extensions of Adversarial Training for Video Classification
Source: arXiv:2206.07953 source file (2022-06-16)
Supplement: Supplementary file 1 [file X_supplementary.tex]

\appendix

% --- PDF will be split by an editor (e.g. macOS preview), so need to restart from page 1
\setcounter{page}{1}

% --- repeat the title (AT: haven't found a more elegant way to do this...)
\twocolumn[
\centering
\Large
\textbf{Analysis and Extensions of Adversarial Training for Video Classification} \\
\vspace{0.5em}Supplementary Material \\
\vspace{1.0em}
] %< twocolumn
\appendix
This Appendix provides additional implementation details (Section ~\ref{sup:exp_impl}), additional experimental details (Section ~\ref{sup:exp_detail}) and an extra experiment (Section ~\ref{sup:extra_exp}), to supplement our main submission. These are not included in the main paper due to space constraints.

\section{Implementation details}
\label{sup:exp_impl}
% This section provides additional implementation and experimental setup details for all the results reported in the experimental results of the main paper.
We use 3D ResNeXt-101 network~\cite{Hara2018CanS3}, as a backbone for the action recognition task and we simply adopt the training strategy and the configuration of parameters from~\cite{Kataoka2020WouldMD}\footnote{\url{https://github.com/kenshohara/3D-ResNets-PyTorch}}. 

\textbf{Inputs.} Training samples are randomly generated from the UCF-101~\cite{Soomro2012UCF101AD}\footnote{\url{https://www.crcv.ucf.edu/data/UCF101.php}} training dataset followed by data augmentation. Temporal position in a given video is selected via uniform sampling to generate the training samples. Thus, an input video is cropped to image sequences of $16$ frames where each frame consists of $112 \times 112$ pixels with $3$ color channels. If a video is shorter than 16 frames, then it is adjusted by looping it as many times as necessary. Next, the training data is augmented by applying random spatial cropping selected from the four corners or the center and their horizontal flipping with $50\%$ probability. The video clips are also scaled by multiplying $\{1, \frac{1}{2^{1/4}}, \frac{1}{\sqrt{2}}, \frac{1}{2^{1/4}}, \frac{1}{2} \}$.

\textbf{Model.} We adopt a 3D CNN architecture based on residual networks (ResNets)~\cite{He2016DeepRL}, as a backbone for the action recognition task. ResNets
% are one of the most successful architectures in the image domain and have achieved state-of-the-art results in many tasks. 
basically provide shortcut connections that allow to bypass a signal from one layer to the next, thus, easing the training of very deep networks. In all experiments, we use 3D ResNeXt-101  network~\cite{Hara2018CanS3}, which performs 3D convolution and 3D pooling. The details of the network architecture is presented in \Table{3d_resnet}. The convolutional kernels are of size $3\times3\times3$ and a temporal stride of $1$ and spatial stride of $2$ is used in $conv1$. The network expects 16-frame video clips as inputs. Spatial down-sampling is performed by $conv1$ and spatio-temporal down-sampling is performed by $conv3\_x$, $conv4\_x$, $conv5\_x$ with a stride of $2$. We also present the details of the generator and discriminator networks of the proposed 3D APE-GAN method in \Table{3d_ape_net}. The convolutional kernels are $4\times4\times4$ with a stride of $2$ and padding of $1$. 
\begin{table}[h]
\centering
% \resizebox{\linewidth}{!}{ %< auto-adjusts font size to fill line
\caption{\textbf{ResNeXt-101 network architecture.} Here, all residual blocks are shown in square brackets and each covolutional layers are followed by batch normalization~\cite{Ioffe2015BatchNA} and ReLU~\cite{Nair2010RectifiedLU} activation function. Spatial down-sampling of input is first performed by $conv1$ (stride $2$). A $3\times3\times3$ max-pooling with a stride of $2$ is then applied before $conv2\_x$. Spatio-temporal down-sampling is performed by $conv3\_x$, $conv4\_x$, $conv5\_x$ with a stride of $2$. The dimension of the last fully-connected layer is set for the UCF-101 dataset. }
\begin{adjustbox}{max width=\linewidth}
\begin{tabular}{cc}
\toprule
{Layer Name}              & {Architecture}              \\
\midrule \midrule
                        & $7\times7\times7$, 64 \\ 
 $conv1$                  & temporal stride 1 \\ 
                        & spatial stride 2 \\ \midrule

                 & $3\times3\times3$ max pool, stride 2 \\
$conv2\_x$        &  $\begin{bmatrix}
                            3\times3\times3, 128\\
                            3\times3\times3, 128
                        \end{bmatrix} \times 3$ \\ \midrule

$conv3\_x$                 & $\begin{bmatrix}
                           3\times3\times3, 256\\
                            3\times3\times3, 256
                        \end{bmatrix} \times 4$ \\ \midrule

$conv4\_x$                 &  $\begin{bmatrix}
                            3\times3\times3, 512\\
                            3\times3\times3, 512
                        \end{bmatrix} \times 23 $ \\ \midrule

$conv5\_x$                 & $\begin{bmatrix}
                            3\times3\times3, 1024\\
                            3\times3\times3, 1024
                        \end{bmatrix} \times 3 $ \\\midrule

\multicolumn{2}{c}{global average pool} \\ \midrule
\multicolumn{2}{c}{101-d fully-connected, softmax} \\
\bottomrule
\end{tabular}
\end{adjustbox}

\label{tab:3d_resnet}
\end{table}
\begin{table}[h]
\centering
% \resizebox{\linewidth}{!}{ %< auto-adjusts font size to fill line
\caption{\textbf{3D APE-GAN network architecture.} The generator and discriminator architecture of the 3D APE-GAN network. Here, conv denotes convolutional layers while deconv denotes layes with transposed convolution operators. All covolutional, transposed convolutional, and fully connected layers but final layers are followed by batch normalization and Leaky ReLU~\cite{Maas2013RectifierNI} activation function. \textit{Generator.} Down-sampling of inputs is first performed by conv1, conv2, and conv3 layers and then it is up-sampled by deconv1, deconv2, and deconv3 layers -- all with a stride of 2 and padding of 1. \textit{Discriminator.} The input is down-sampled by all the convolutional layers followed by a fully connected layer to result in 1024-d. A final fully connected layer with a sigmoid activation function is then applied to obtain the prediction of the class.}
\begin{adjustbox}{max width=\linewidth}
\begin{tabular}{llll}
\toprule
% \multicolumn{4}{c}{3D APE-GAN} \\ \midrule
\multicolumn{2}{c}{Generator} & \multicolumn{2}{c}{Discriminator} \\ \midrule
{Layer Name}     & {Architecture}   & {Layer Name}       & {Architecture}   \\
\midrule \midrule
conv1                   & $4\times4\times4$, 64                 & conv1                     &  $4\times4\times4$, 64 \\ \hline
conv2                   & $4\times4\times4$, 128                & conv2                     &  $4\times4\times4$, 128 \\ \hline
conv3                   & $4\times4\times4$, 256                & conv3                     &  $4\times4\times4$, 256 \\ \hline
deconv1                 & $4\times4\times4$, 256                & conv4                     &  $4\times4\times4$, 512 \\ \hline
deconv2                 & $4\times4\times4$, 128                & \multicolumn{2}{c}{1024-d fully-connected} \\ \hline
% & \midrule
deconv3, sigmoid & $4\times4\times4$, 3                  & \multicolumn{2}{c}{1-d fully-connected, sigmoid} \\
\bottomrule
\end{tabular}
\end{adjustbox}

\label{tab:3d_ape_net}
\end{table}

\textbf{Training.} To train the 3D ResNeXt-101 network on the UCF-101 dataset, we use stochastic gradient descent (SGD)~\cite{Kiefer1952StochasticEO} optimizer, having an initial learning rate of $0.1$, decayed if the validation loss is saturated for $10$ epochs in a row. However, an initial learning rate of $5e-4$ is used in the case of adversarial training. A weight decay of $1e-3$ and momentum of $0.9$ is used in the standard training, while the weight decay is set to $1e-5$ in adversarial training. On the other hand, we train the 3D APE-GAN network on the same dataset with the Adam~\cite{Kingma2015AdamAM} optimizer, having a learning rate of $2e-4$ and initial decay rates of $0.5, 0.999$ for the first and second moments of the gradient, respectively.

\textbf{Evaluation} We evaluate our model (the checkpoint at the end of training) on the UCF-101 dataset. We use the top-1 video-level accuracy as an evaluation metric. It is computed by accumulating the probability of video clips in the video, where non-overlapped sliding window method is used to output probability using the trained network.

\section{Additional experimental details}
\label{sup:exp_detail}
In this section we provide additional details about the attack parameters used in the experiment reported in Figure 5 of the main paper. 
In the frame saliency attacks, both one-shot and iterative, an $\ell_\infty$ PGD attack of 100 steps with step size $\alpha=0.102$ is applied, whereas an $\ell_\infty$ PGD attack of 300 steps with an attack budget of $\epsilon=255$ and step size $\alpha=0.1275$ is used in both masked PGD and frame border attacks. For the flickering attack, $100$ steps of attacks with step size of $5$, loss margin of 0.05, and $\beta_1=0.1$, $\beta_2=0.9$ weighting the thickness and roughness regularization, respectively, is used. Moreover, even though the model was evaluated on three different attack strength of each method, the training was only performed on one attack strength from all attack methods but flickering. Therefore, the network was trained with attack budget of $\epsilon=2$ in both frame saliency attacks, and with patch ratio of $r=0.15$ in masked PGD and frame border attacks.

\section{Extra experiments}
\label{sup:extra_exp}
All the experiments in main paper are evaluated with $5$ steps of optimal PGD attacks at test time. In this section, we present evaluation of the same methods on sub-optimal PGD attacks. \Table{suboptim_attack} shows the robust performance of the different methods against weak PGD attacks (with step size of $\alpha=\frac{\hat{\alpha}}{2}$) at test time. From the results, we can see that all the methods are more robust to weaker attacks compared to strong attacks as one would expect. The result gap between robustness against strong and weak attacks also suggests that the need to finetune the attack parameters to generate a strong attack at test time in order to avoid a false sense of robustness. From the result, we can still see that adversarial training with optimal and strong attacks perform worse than adversarial training with weaker attacks. Moreover, we can see that all the proposed methods improve the robustness in the same way as in the case of optimal attacks. 

\begin{table}[th]
\centering
% \resizebox{\linewidth}{!}{ %< auto-adjusts font size to fill line
\caption{
\textbf{Performance against weaker attacks} -- robust performance of models trained with different variations of AT and 3D APE-GAN. All attacks are computed via PGD $\ell_\infty$ with sub optimal step size, specifically $\frac{\hat{\alpha}}{2}$, and the results are top-1 test accuracy. $AAT$ with attack budget $\epsilon=auto$ represents the adaptive random sampling method of variable attack budgets. $CAT$ indicates a curriculum training with $\epsilon=\uparrow_0^{12}$, i.e. an increasing attack budget from $\epsilon=0$ to $\epsilon=12$. APE denotes the proposed 3D APE-GAN method using benign action recognition network, while $GAT$ represents the Generative AT, i.e. end-to-end adversarial training of both 3D APE-GAN and action recognition network.
} % \caption
\begin{adjustbox}{max width=\linewidth}
\begin{tabular}{@{}llllll@{}}
\toprule
\multicolumn{1}{c}{\multirow{2}{*}{Model}} & \multicolumn{5}{c}{Evaluation Attack} \\
                   & $\epsilon=0$ & $\epsilon=4$ & $\epsilon=8$ & $\epsilon=12$ & $\epsilon=15$ \\\midrule
\midrule
Benign                                      & {92.3}     & 04.5          & 02.4          & 02.1          & 01.9          \\ \midrule
$AT(\epsilon=8,\alpha=\hat{\alpha})$        & 28.8              & 23.9          & 19.2          & 17.3          & 16.2    \\
$AT(\epsilon=8,\alpha=\frac{\hat{\alpha}}{2})$ & \textbf{72.9}  & \textbf{51.3} & 36.8	        & 28.7      	& 26.6    \\
$AT(\epsilon=8,\alpha=\epsilon)$            & 64.1              & {49.9}        & \textit{36.9} & \textbf{30.8} & \textbf{29.2} \\
$AT(\epsilon=4,\alpha=\epsilon)$            & \textit{70.1}     & \textit{51.1} & \textbf{38.2} & \textit{29.9} & \textit{27.0}    \\
$AT(\epsilon=12,\alpha=\epsilon)$           & 34.3              & 27.9          & 23.6          & {21.0}        & {20.1} \\
\midrule
$AAT(\epsilon=auto,\alpha=\epsilon)$        & \textit{54.5}     & \textit{46.3}	        & \textit{37.4}	    & \textit{32.0}	    &	\textit{29.9} \\
$CAT(\epsilon=\uparrow_0^{12},\alpha=\epsilon)$ & \textbf{61.1} & \textbf{48.3} & \textbf{38.7} & \textbf{34.2} &	\textbf{32.6} \\
\midrule
$APE(\epsilon=\uparrow_0^{12},\alpha=\epsilon)$ & \textbf{81.6} & \textit{71.0} & \textit{61.1}	& \textit{57.4}	& \textit{55.9} \\
$GAT(\epsilon=8,\alpha=8$)                   & \textit{81.1}    & \textbf{73.5}	& \textbf{65.1}	& \textbf{61.1} & \textbf{59.8}  \\
\bottomrule
\end{tabular}
% } %< \resizebox
\end{adjustbox}

\label{tab:suboptim_attack}
\end{table}

% \subsection{Computational efficiency}
% \label{sup:exp_runtime}
% All models were implemented in Python using Pytorch 1.2.0 and are 
% based on the Grounded Video Description open-source code. As mentioned before, our GVD-CVAE does not add any computational cost to GVD. Given pre-extracted video and region features, a forward pass through our model for 20 ActivityNet videos (10 frames sampled from each, $M=1000$) takes 0.7 seconds at a single Tesla K80 GPU. We train our models on 4 GPUs and training lasts from around 6 to 12 hours depending on the model.
